# Supplementary material for: Towards Quantum Computational Mechanics
Source: arXiv:2312.03791 source file (2024-10-07)
Supplement: Supplementary file 1 [file appendix.tex]

\begin{comment}
%
%--------------------------------------------------------------------------------
\section{Kronecker Product}
%--------------------------------------------------------------------------------
%
The Kronecker product satisfies the following properties. 
%
\begin{enumerate}
	\item $ (A \otimes C) (B \otimes D) = AB \otimes CD $
	\item $ (A \otimes C)  ( \ket u \otimes \ket w) = A \ket u \otimes C \ket w $
	\item $  (\ket u + \ket v) \otimes \ket w = \ket u \ket w \otimes \ket v \otimes \ket w$
	\item $ \ket u \otimes (\ket w + \ket x) =  \ket u \otimes \ket w + \ket u \otimes  \ket x  $ 
	\item $a \ket u \otimes b \ket w = ab \ket u \otimes \ket w$ 
	\item $(A \otimes B)^\dagger = A^\dagger \otimes B^\dagger $
\end{enumerate}
%
\end{comment}

\begin{comment}
%
%-------------------------------------------------------------------------------- 
\section{Complexity of the polynomial encoding algorithm}
\label{sec:Poly complexity}
%--------------------------------------------------------------------------------
%
We provide an estimate of the computational complexity of the polynomial encoding circuit. Note from \ref{eq:2D Polynomial} that the number of terms in $(2^{n-1}k_{n-1}+...+2^1k_1+2^0k_0)^m$ for a fixed $m$ equals $
\binom{n+m-1}{n-1}$. The total number of terms with varying $m \in \{0,1,..., p\}$ can be computed as 
\begin{equation} 
\label{eq: sum multinomial}
\binom{n-1}{n-1}+\binom{n}{n-1}+\binom{n+1}{n-1}+...+\binom{n+p-1}{n-1}. 
\end{equation}
Recall, for any $r \in \{0,...,n\}$,
\begin{equation}
\binom{n}{r}+\binom{n}{r+1}=\binom{n+1}{r+1}. 
\end{equation}
We conclude that the sum in \ref{eq: sum multinomial} equals
\begin{equation}
\begin{split}
    &\binom{n-1}{n-1}+\binom{n}{n-1}+\binom{n+1}{n-1}+...+\binom{n+m-1}{n-1} = % \\ & =
    \binom{n}{n}+\binom{n}{n-1}+\binom{n+1}{n-1}+...+\binom{n+p-1}{n-1} 
    = \\ & 
    \binom{n+1}{n}+\binom{n+1}{n-1}+...+\binom{n+p-1}{n-1} 
    = % \\ & = 
    \binom{n+p}{n} .
\end{split}
\end{equation}
Therefore, for one-dimensional and two dimensional polynomial encoding we conclude that we need a total of $\binom{n+p}{n}$ and $\binom{n+p}{n}\binom{n+q}{n}$  multi-controlled $R_Y$ gate, respectively. Overall, we conclude that the polynomial encoding can be implemented with $\mathcal{O} \ (\textrm{Poly } (pn))$ in single variate polynomials of order and $\mathcal{O} \ (\textrm{Poly } (pqn^2))$ for bi-variate polynomials. 
\end{comment}
